# Supplementary material for: Exploiting spatiotemporal degrees of freedom for far field subwavelength focusing using time reversal in fractals
Source: arXiv:1603.01725 source file (2016-03-05)
Supplement: Supplementary file 1 [file Supplemental_Material_Dupre.pdf]

# Supplemental Material: Exploiting spatiotemporal degrees of freedom for far field subwavelength focusing using time reversal in fractals

Matthieu Dupré[1], Fabrice Lemoult[1], Mathias Fink[1], Geoffroy Lerosey[1]

[1]Institut Langevin, ESPCI ParisTech & CNRS, 1 rue Jussieu 75005 Paris, France

## 1) Simulations parameters

Simulations have been performed with a FDTD method (CST microwave studio). The dimensions of the simulated Hilbert fractal of order 6 correspond to the real one with a footprint of 120 mm, a width of 0.75 mm and a thickness of 30 µm. The metal is lossless, but the FR4 substrate (thickness 1.5 mm) is simulated with its commercial properties in terms of index and loss ($\tan\delta=3.10^{-2}$). We do not use any cavity in simulations.

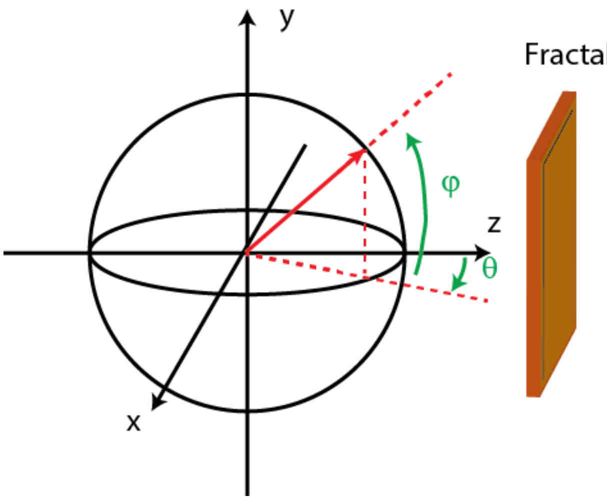


**Figure S1 Geometry of the simulations. Definition of angles θ and φ.**

The geometry and the incident angles of plane waves are defined on figure S1. We run 90 simulations for 45 incident angles (5 angles for $\theta$ included between 0 and 84° and 9 angles for $\varphi$ between -84 and 84°. Indeed, the right-left symmetry of the fractal does not require exciting it with both positive and negative $\theta$ angles. Each incident **k** vector is simulated twice for the two orthogonal polarizations.

The plane wave is a Gaussian pulse which frequencies are included between the 1.5 GHz and 3 GHz bandwidth. The signal is recorded by steps of 0.1 ns from 0 to 500 ns, at which time the energy in the simulated domain is 20 dB under its maximum value.

The **z** polarization of the electric field is recorded at 1 mm of the fractal. It is spatially convolved by the measured transfer function (averaged on the bandwidth) of the probe used to do the measurement. Its effect amounts to average the field on a few squared millimeters, which amounts to a few pixel sizes, as we can see on the figure S2. The simulated signal of the plane wave *n* at a position ***r*** in the fractal near field and time *t* is therefore given by:

$$s_n(\boldsymbol{r}, t) = E_z(\boldsymbol{r}, t) *_r H(\boldsymbol{r})$$

where $*_r$ stands for the spatial convolution. The time reversed field at ***r*** when trying to focus a position $\boldsymbol{r_0}$ is therefore given by:

$$s_{TR}(\boldsymbol{r}, \boldsymbol{r_0}, t) = \sum_{n=1}^{N=90} s_n(\boldsymbol{r}, t) *_t s_n(\boldsymbol{r_0}, -t)$$

where $*_t$ stands for the temporal convolution operation.

## 2) Measure of the probe transfer function

*H* is measured experimentally, by measuring the transmission $T(\boldsymbol{r}, f)$ between two identical near field probes. One is scanned at 0.5 mm of the other in a 120 by 120 mm$^2$ area in the 1.5 GHz-3GHz bandwidth

with a frequency sampling of 1 MHz. There are therefore $N$=1501 measured frequencies. This transmission is averaged over the frequencies to get $T_m(\boldsymbol{r}) = \frac{1}{N}\sum_f T(\boldsymbol{r}, f)$. However this is the auto-convoluted transfer function of the probe. Therefore we deconvolute it using Fourier transforms to get the real transfer function (Fig. S2):

$$H(\boldsymbol{r}) = \mathcal{F}^{-1}\left[\sqrt{\mathcal{F}[T_m(\boldsymbol{r})]}\right]$$

where $\mathcal{F}$ stands for the Fourier transform.

The effect of H is mainly to average the field measured of a small area of a few mm².

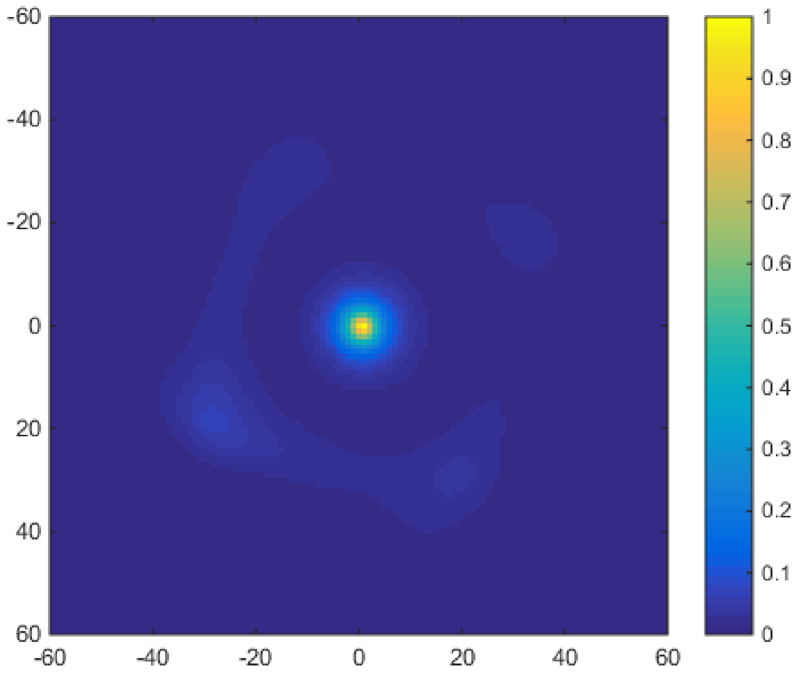


**Figure S2. Transfer function (au) of the measurement probe (averaged in frequency on the 1.5-3GHz bandwidth).**

## 3) Number of degrees of freedom in simulations

The simulations provide 90 electric fields digitized on 120 mm² x 120 mm² per 50.1x0.1 ns. In order to evaluate the number of degrees of freedom, we compute the spatial and temporal coefficient of correlations of the 90 incident waves $\alpha$.

$$\begin{cases} R_s(\alpha_i, \alpha_j) = \left\langle \dfrac{\left|\sum_{\boldsymbol{r}} E_{\alpha_i}(\boldsymbol{r},t) E_j(\boldsymbol{r},t)\right|}{\sqrt{\sum_{\boldsymbol{r}} \left|E_{\alpha_i}(\boldsymbol{r},t)\right|^2 \sum_r \left|E_{\alpha_j}(\boldsymbol{r},t)\right|^2}} \right\rangle_t \\ R_t(t_i, t_j) = \left\langle \dfrac{\left|\sum_t E_\alpha(\boldsymbol{r},t_i) E_\alpha(\boldsymbol{r},t_j)\right|}{\sqrt{\sum_t |E_\alpha(\boldsymbol{r},t_i)|^2 \sum_r \left|E_\alpha(\boldsymbol{r},t_j)\right|^2}} \right\rangle_\alpha \end{cases}$$

The rows of each matrix are then sorted and their lines are averaged to get the average correlation coefficients between those antennas. The number of spatial degrees of freedom is given by the total number of antennas (90) divided by the number of correlated fields (for which the average correlation coefficient is above 0.5), that is 90/9=10 spatial degrees of freedom. We can see that the two polarizations are uncorrelated as on Fig.S3 (a), while the plane waves with close angles are correlated, which produces the high correlated diagonals on Fig.S3 (a).

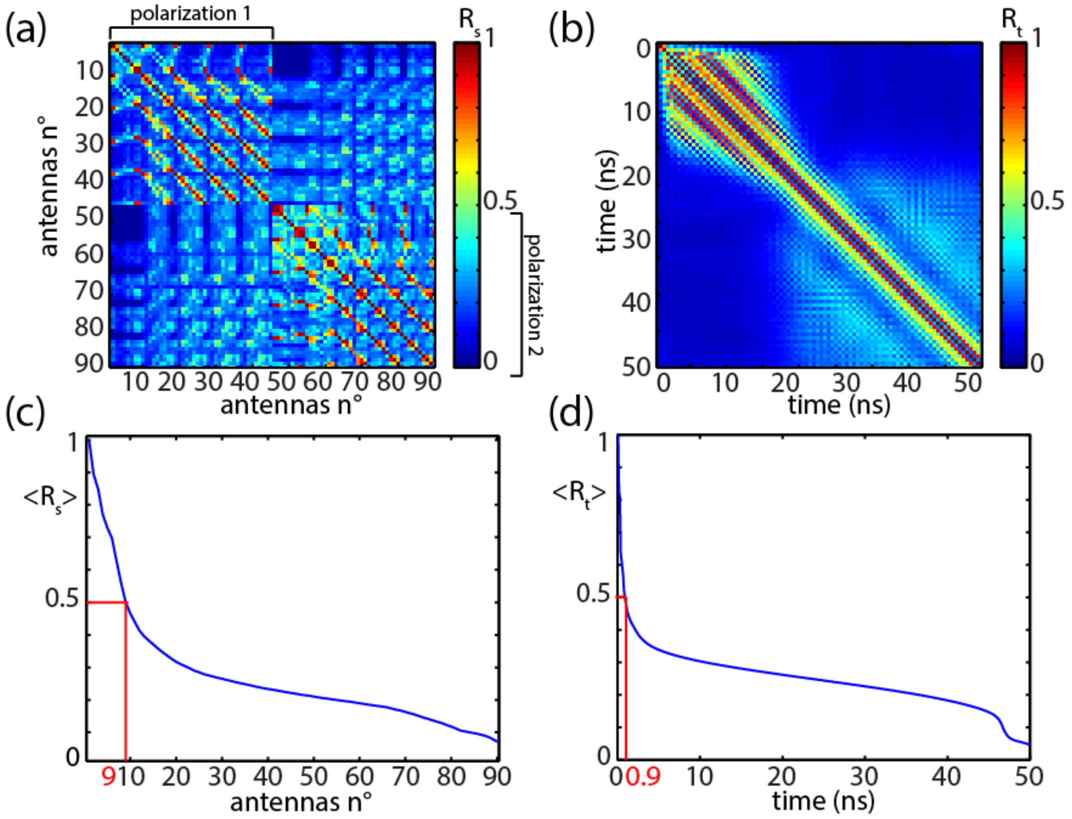


**Figure S3. (a) Matrix of the coefficients of correlation of the spatial degrees of freedom. (b) Idem for the temporal degrees of freedom. (c) Averaged spatial correlation coefficients. (d) Averaged temporal correlation coefficients**

The number of temporal degrees of freedom is given by:

$$N_t = \frac{\Delta \mathrm{T}}{\delta t} = 22$$

where $\Delta \mathrm{T}$ is the characteristic life time of the resonances of the fractal, and $\delta t$ the time of coherence. Logically, $\delta t$ which has been measured to be 0.9 ns is superior to the duration of the pulse (0.5 ns at 2 GHz). $\Delta \mathrm{T}$ is measured around 20 ns for our simulations We can compare it to the measured one in experiment which is 15 ns for the measurements obtained with one antenna. Those values are consistent as in experiment the metal of the fractal is not perfect and adds additional dissipation. Hence the number of temporal degrees of freedom is 22.

The total number of degrees of freedom is therefore $N_{tot} = N_s N_t = 220$.

## 4) Number of degrees of freedom in experiments

We do the exact same procedure in experiment, but counting only the temporal degrees of freedom as we have only one emitter in this case. Moreover this time the calculation is performed in the frequency domain. We have a bandwidth of $\Delta f = 1.5$ GHz (from 1.5 to 3 GHz). We measure without a cavity a correlation frequency of $\delta f =$122 MHz for 9 MHz with a cavity. This provides respectively $N_t$=12 temporal degrees of freedom without a cavity for $N_t$=150 with it. The number of degrees of freedom without a cavity is of the same order than the total numbers of degrees of freedom obtained in simulations, however a little lesser. This decreased number could be attributed to the metallic losses that where neglected in simulations where we have used PEC to simulate the fractal resonator.

The number of temporal degrees of freedom without a cavity is almost the same in experiment and simulations which is consistent.

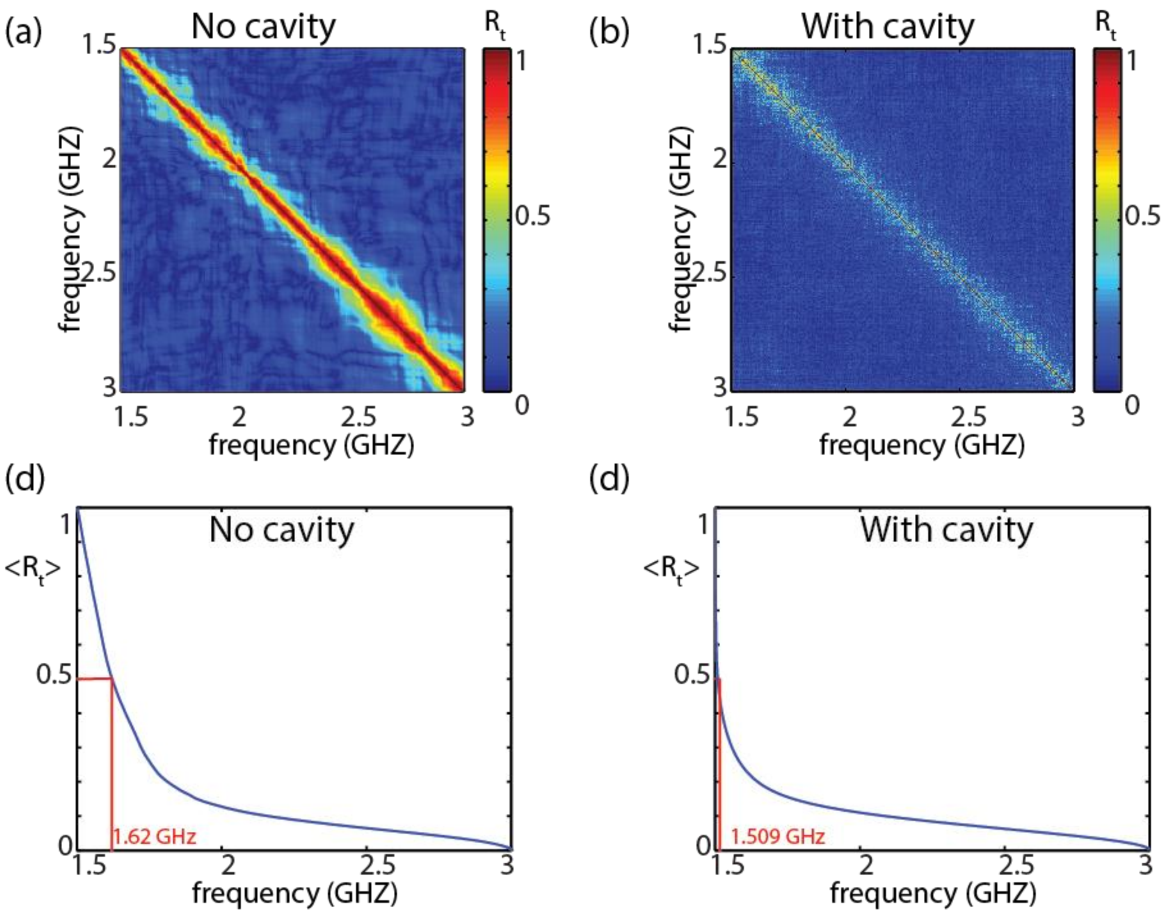


**Figure S4. Calculation of the correlation frequency. (a) frequency to frequency correlation coefficients for the measurement without a cavity. (b) Idem with a cavity. (c) Averaged correlations coefficients without a cavity. (d) Idem with a cavity.**

## 5) Simulation results

We obtain 100 focal spots at random positions. Thereafter, we present nine of them alongside with the corresponding TR focal spots obtained either in experiment with one antenna from the far field or with a cavity backed to the fractal, or either in simulations with 90 plane waves (45 incident angles and 2 orthogonal polarizations).

Qualitatively, figures S5-7 indicate that focusing with a cavity provides slightly better results than with 90 plane waves, which in their turn provide a much better focusing than with a single antenna. We can note an exception on the Figure S6 with the focal spot n°4, as with a cavity an additional hot spot is lighted. The case number 1) on Fig. S5 is also an exception as the three procedures provide a good focusing.

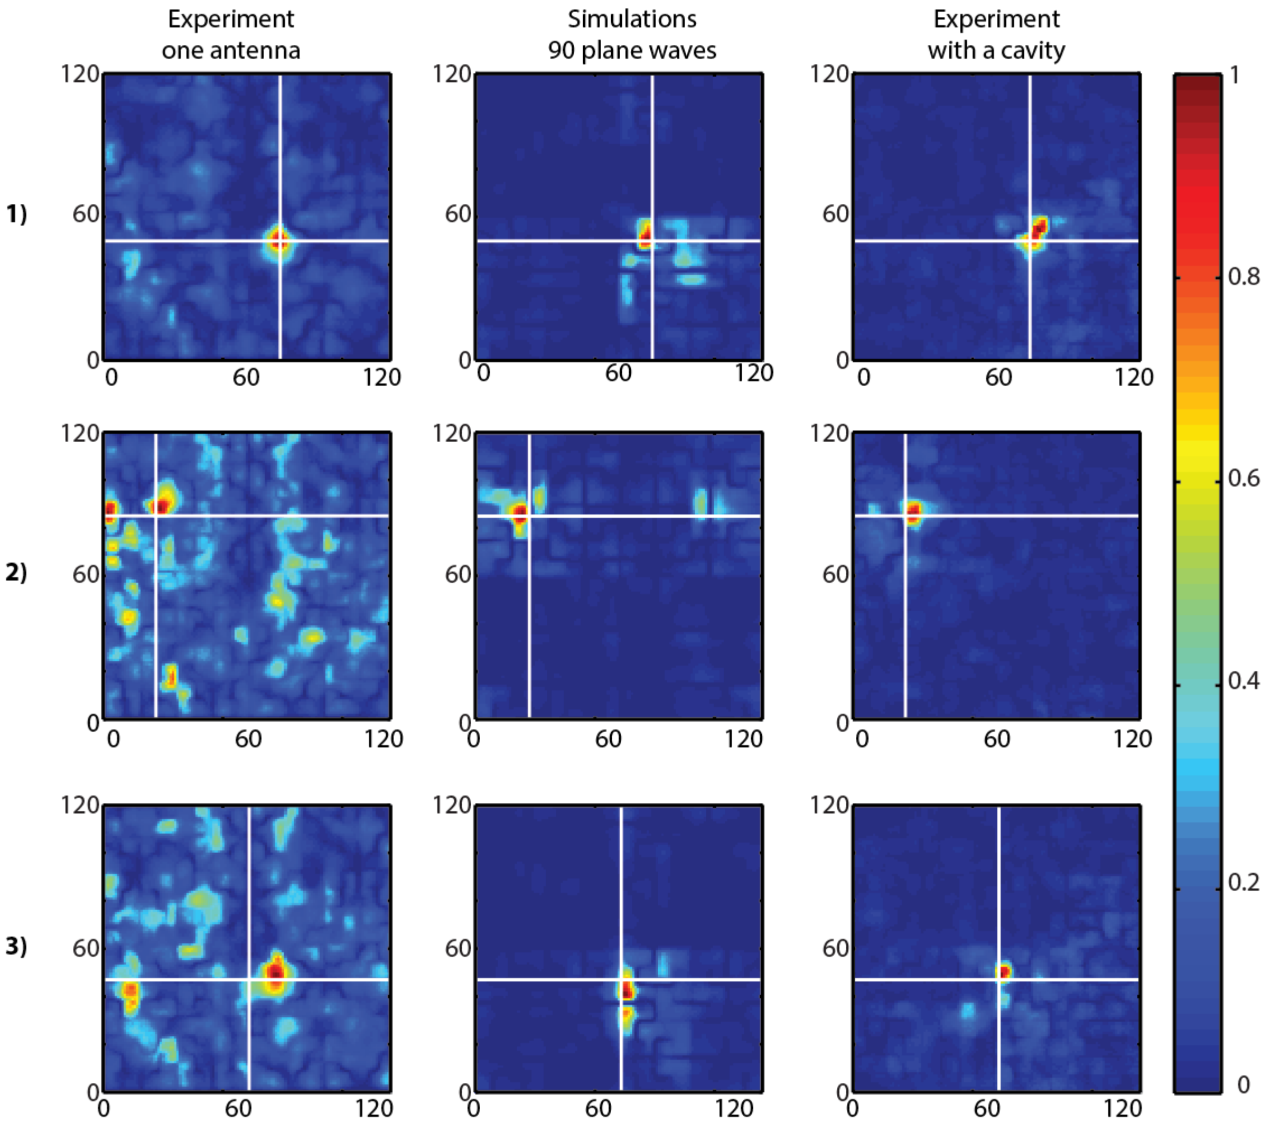


**Figure S5. Comparison of focal spots obtained in experiments and simulations.**

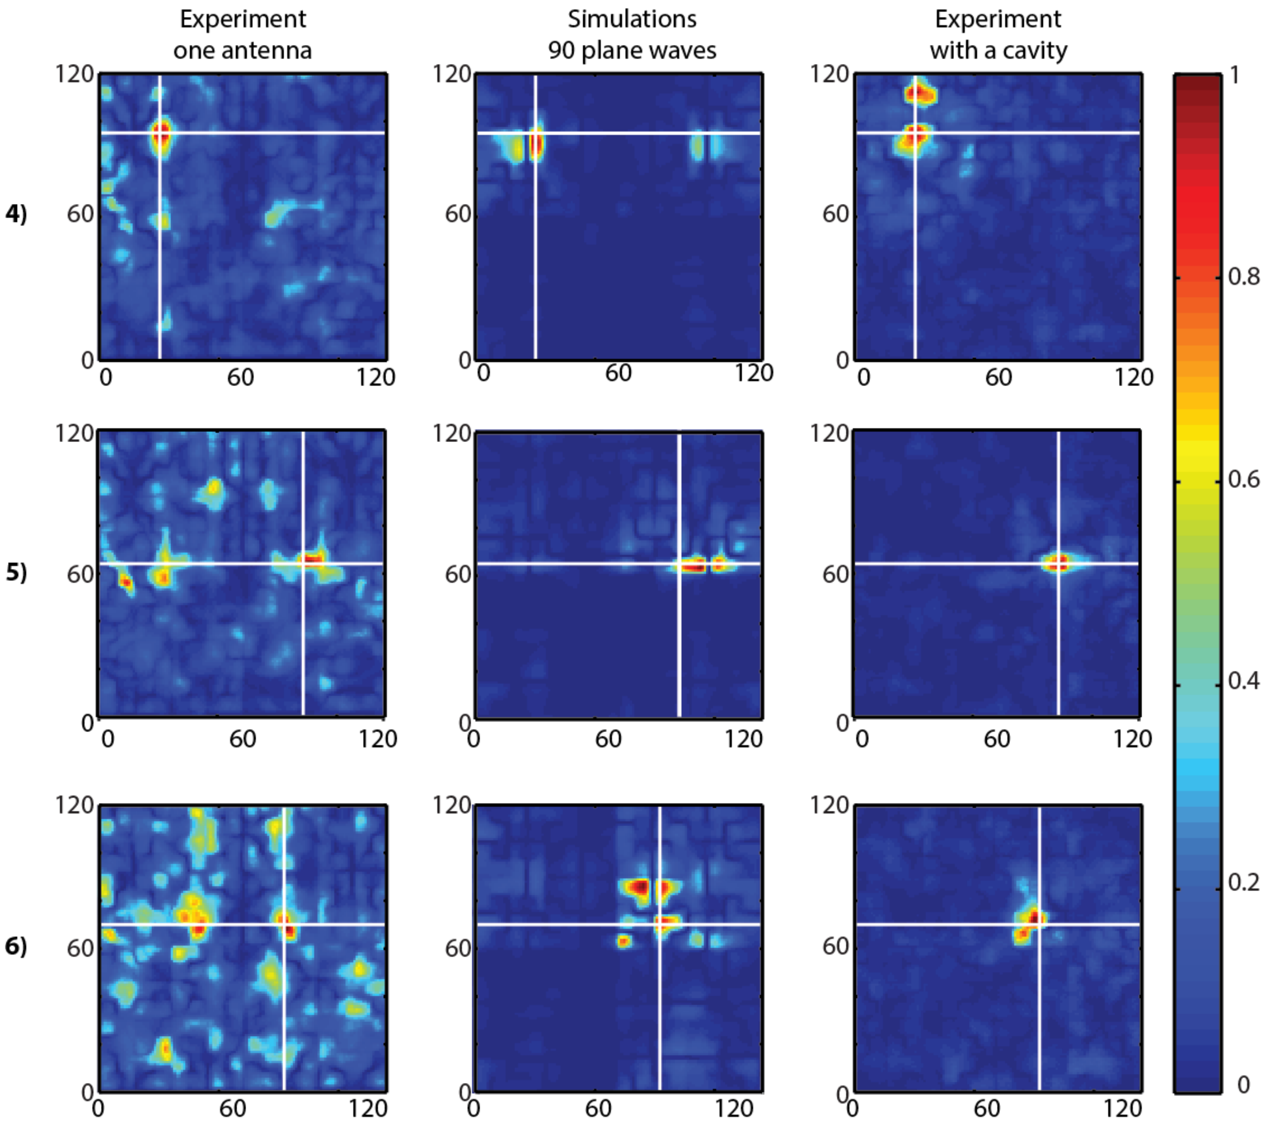


Figure S6. Comparison of focal spots obtained in experiments and simulations.

We can also notice that with only one antenna, there is in general a very high background with a low SNR, and that the excited hot spot can be far away from the targeted one. Simulations with 90 plane waves provide better results in terms of SNR: only a few hot spots in the vicinity of the target are excited.

Finally, the experimental results obtained with a cavity are much better in terms of SNR and error to the target.

In general the sizes of the focal spots appear to be of the same order of magnitude for the different configurations.

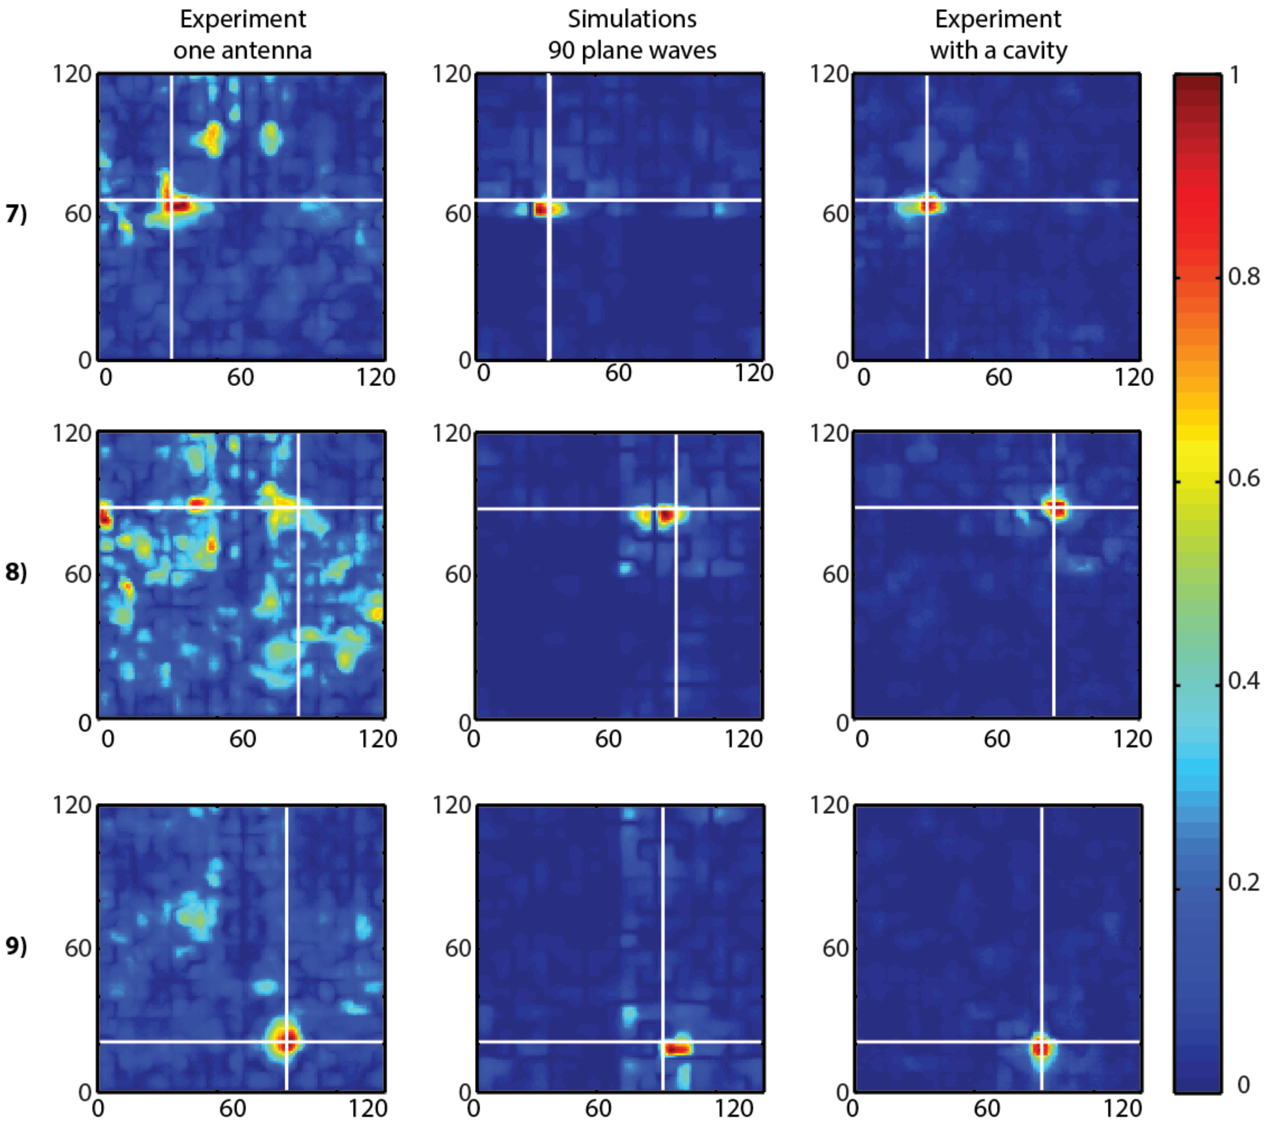


Figure S7. Comparison of focal spots obtained in experiments and simulations.

## 6) Comparison of the results

The simulations aim at comparing the improvement of using a cavity that increases the temporal degrees of freedom by approximately 12.5, to the increase of spatial degrees of freedom.

We can look at different parameters as figures of merit to compare the difference between the 90 antennas in simulations or the measurements with one antenna or one cavity. Namely we will compare the average size of the focal spot (Fig.S8 (a)), the spatial signal to noise ratio (SNR) (Fig.S8 (c)), and the

average error between the real and the targeted positions of the focal spots(Fig.S8.(b)). All those numbers are averaged over 100 focusing experiments (or simulations), 9 of which are presented on Fig. S5-7.

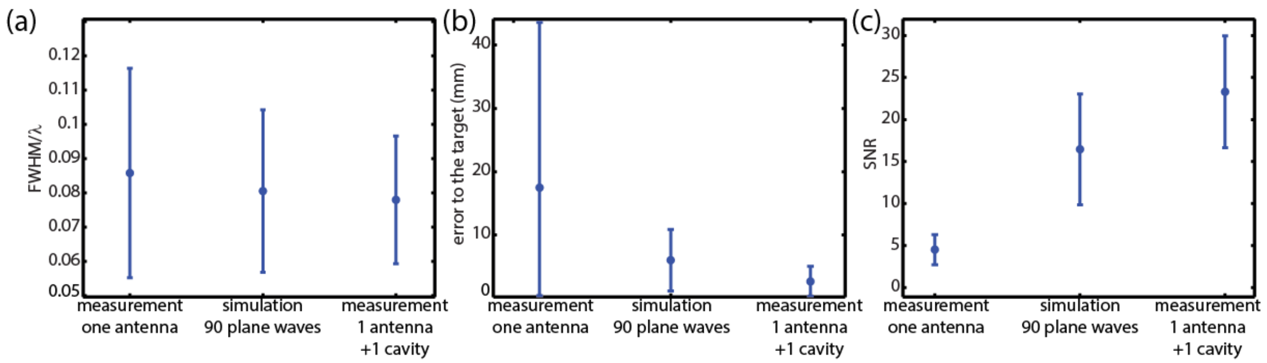


Figure S8. Statistics of the focal spots in experiments and simulations. The error bars show the standard deviation. (a) Average size of the focal spot. (b) Error to the targeted position of the focal spot. (c) Spatial SNR

Even if the average size of the focal spots is only slightly better with a cavity than with only one antenna, the standard deviation with a cavity is much smaller. Thence the sizes of the focal spots are more homogeneous, which is important in terms of applications.

We can also see that the error in terms of location of the focal spot is quite important with only one antenna: the excited hot spots can be anywhere on the fractal (Fig.S6 (b)). With an increased number of spatial degrees of freedom his error is reduced and hot spots in the vicinity of the target are lighted. With a cavity he error in terms of the position of the focal spots is better, reaching 1-2 mm which almost to corresponds to the discretization steps of the measurements (1 mm).

Finally, there is a clear increase of the SNR along with the improvement of the number of degrees of freedom. It is close to zero with a single antenna, which is due to the fact that the targeted position receives a lower energy than the average background, the latter mainly due to the hot spots far-away from the target. On the contrary the SNR is much higher when using 90 antennas for time reversal or a cavity.

All in all, those results are consistent with the evaluated numbers of degrees of freedom, even if it is not completely clear why the experimental focusing with a cavity is slightly better than with 90 plane waves although we have computed a lesser number of degrees of freedom.
